# Supplementary material for: Quantum spin dynamics
Source: arXiv:1410.6383 ancillary file (2014-10-23)
Supplement: Supplementary file 1 [file Supplement.pdf]

# Supplement: Quantum spin dynamics

R. Wieser
*Institut für Angewandte Physik und Zentrum für Mikrostrukturforschung, Universität Hamburg, Jungiusstrasse 11, D-20355 Hamburg, Germany*
(Dated: September 29, 2014)

PACS numbers: 75.78.-n, 75.10.Jm, 75.10.Hk

## I. DERIVATION OF THE LANDAU-LIFSHITZ EQUATION FOR $S = 1$

To prove the given statement that only the vector term $\sum_m \langle \hat{S}_m \rangle \hat{S}_m$ of $\hat{\rho}$ will contribute to the description of the dynamics of $\langle \hat{\mathbf{S}} \rangle$ we have to determine the following equation of motion:

$$\mathrm{Tr}\left(\frac{\mathrm{d}}{\mathrm{d}t}\hat{\rho}\hat{S}_n\right) = i\mathrm{Tr}\left([\hat{\rho},\hat{\mathrm{H}}]\hat{S}_n\right) - \lambda \mathrm{Tr}\left([\hat{\rho},[\hat{\rho},\hat{\mathrm{H}}]]\hat{S}_n\right) \ , \tag{1}$$

for a certain $S$ and taking into account all expansion terms of $\hat{\rho}$:

$$\hat{\rho} = \frac{1}{2S+1}\hat{\mathbf{1}} + \frac{1}{n_S}\sum_m \langle \hat{S}_m \rangle \hat{S}_m + \frac{1}{n_{2S}}\sum_{ml}\langle \hat{S}_{ml}\rangle \hat{S}_{ml} + \dots \ . \tag{2}$$

In the following we set $S = 1$, which means $\hat{\rho}$ is given by:

$$\hat{\rho} = \frac{1}{3}\hat{\mathbf{1}} + \frac{1}{2}\sum_m \langle \hat{S}_m \rangle \hat{S}_m + \frac{1}{2}\sum_{ml}\langle \hat{S}_{ml}\rangle \hat{S}_{ml} \ . \tag{3}$$

An extension to $S > 1$ will lead to the same results. In the case of $S = 1/2$ the bivector term $\sum_{ij}\langle \hat{\sigma}_{ij}\rangle \hat{\sigma}_{ij}$ is already zero due to the Clifford algebra, which tells us that $\hat{\sigma}_i\hat{\sigma}_j = -\hat{\sigma}_j\hat{\sigma}_i$ and therefore $[\hat{\sigma}_i, \hat{\sigma}_j]_+ = 0$.

Inserting (3) in (1) gives for the left hand side of (1):

$$\mathrm{Tr}\left(\frac{\mathrm{d}}{\mathrm{d}t}\hat{\rho}\hat{S}_n\right) = \frac{1}{3}\frac{\mathrm{d}\hat{\mathbf{1}}}{\mathrm{d}t}\underbrace{\mathrm{Tr}\left(\hat{S}_n\right)}_{=0} + \frac{1}{2}\sum_m \frac{\mathrm{d}\langle \hat{S}_m\rangle}{\mathrm{d}t}\underbrace{\mathrm{Tr}\left(\hat{S}_m\hat{S}_n\right)}_{=2\delta_{nm}} + \frac{1}{2}\sum_{ml}\frac{\mathrm{d}\langle \hat{S}_{ml}\rangle}{\mathrm{d}t}\underbrace{\mathrm{Tr}\left(\hat{S}_{ml}\hat{S}_n\right)}_{=0} \ . \tag{4}$$

With aid of the rule:

$$\mathrm{Tr}\left(\hat{S}^k_\alpha \hat{S}^{k'}_\beta\right) = n_{S_k}\delta_{\alpha\beta}\delta_{kk'} \ , \tag{5}$$

and the fact that the spin matrices $\hat{S}_n$ are traceless: $\mathrm{Tr}\left(\hat{S}_n\right) = 0$ we find for the left hand side of (1) the expected result:

$$\mathrm{Tr}\left(\frac{\mathrm{d}}{\mathrm{d}t}\hat{\rho}\hat{S}_n\right) = \frac{\mathrm{d}}{\mathrm{d}t}\langle \hat{S}_n\rangle \ . \tag{6}$$

After inserting (3) in (1) the first term $i\mathrm{Tr}\left([\hat{\rho},\hat{\mathrm{H}}]\hat{S}_n\right)$ on the right hand side of (1) becomes:

$$i\mathrm{Tr}\left([\hat{\rho},\hat{\mathrm{H}}]\hat{S}_n\right) = -\frac{i}{3}\sum_a B^a_{\mathrm{eff}}\mathrm{Tr}\left([\hat{\mathbf{1}},\hat{S}_a]\hat{S}_n\right) - \frac{i}{2}\sum_{ma}\langle \hat{S}_m\rangle B^a_{\mathrm{eff}}\mathrm{Tr}\left([\hat{S}_m,\hat{S}_a]\hat{S}_n\right) - \frac{i}{2}\sum_{mla}\langle \hat{S}_{ml}\rangle B^a_{\mathrm{eff}}\mathrm{Tr}\left([\hat{S}_{ml},\hat{S}_a]\hat{S}_n\right) \tag{7}$$

Here, we have assumed that $\hat{\mathrm{H}}$ is given by:

$$\hat{\mathrm{H}} = -\sum_a B^a_{\mathrm{eff}}\hat{S}_a \ . \tag{8}$$

The first term on the right hand side of (7) is zero because of $[\hat{\mathbf{1}}, \hat{S}_a] = 0$. The trace of the second term becomes:

$$\mathrm{Tr}\left([\hat{S}_m,\hat{S}_a]\hat{S}_n\right) = i\mathrm{Tr}\left(\hat{S}_b\hat{S}_n\right)\epsilon_{mab} = 2i\delta_{bn}\epsilon_{mab} \ , \tag{9}$$

and therefore:

$$-\frac{i}{2}\sum_{ma}\langle\hat{S}_m\rangle B^a_{\text{eff}}\,\text{Tr}\left([\hat{S}_m,\hat{S}_a]\hat{S}_n\right)=\sum_{ma}\langle\hat{S}_m\rangle B^a_{\text{eff}}\epsilon_{man}=\left(\langle\hat{\mathbf{S}}\rangle\times\mathbf{B}_{\text{eff}}\right)_n\ . \tag{10}$$

The commutator in the third term can be written as:

$$[\hat{S}_{ml},\hat{S}_a]=i\left(\hat{S}_{mc}\epsilon_{lac}+\hat{S}_{bl}\epsilon_{mab}\right)\ , \tag{11}$$

and therefore, we get two terms with $\text{Tr}\left(\hat{S}_n\hat{S}_{ml}\right)=0$. This means that the trace of the third term becomes zero. In summary, only the vector term contributes to the description and $i\text{Tr}\left([\hat{\rho},\hat{\text{H}}]\hat{S}_n\right)$ becomes:

$$i\text{Tr}\left([\hat{\rho},\hat{\text{H}}]\hat{S}_n\right)=\left(\langle\hat{\mathbf{S}}\rangle\times\mathbf{B}_{\text{eff}}\right)_n\ . \tag{12}$$

This result has been mentioned in the publication and can be found in [1, 2].

The second term $-\lambda\text{Tr}\left([\hat{\rho},[\hat{\rho},\hat{\text{H}}]]\hat{S}_n\right)$ on the right hand side of (1) is more tricky. Inserting $\hat{\rho}$ [Eq. (3)] and $\hat{\text{H}}$ [Eq. (8)] we get:

$$\begin{aligned}-\lambda\text{Tr}\left([\hat{\rho},[\hat{\rho},\hat{\text{H}}]]\hat{S}_n\right) &= -\frac{\lambda}{4}\sum_{mba}\langle\hat{S}_m\rangle\langle\hat{S}_b\rangle B^a_{\text{eff}}\text{Tr}\left([\hat{S}_m,[\hat{S}_b,\hat{S}_a]]\hat{S}_n\right)-\frac{\lambda}{4}\sum_{mlba}\langle\hat{S}_{ml}\rangle\langle\hat{S}_b\rangle B^a_{\text{eff}}\text{Tr}\left([\hat{S}_{ml},[\hat{S}_b,\hat{S}_a]]\hat{S}_n\right)\\ &-\frac{\lambda}{4}\sum_{bmla}\langle\hat{S}_b\rangle\langle\hat{S}_{ml}\rangle B^a_{\text{eff}}\text{Tr}\left([\hat{S}_b,[\hat{S}_{ml},\hat{S}_a]]\hat{S}_n\right)-\frac{\lambda}{4}\sum_{mluva}\langle\hat{S}_{ml}\rangle\langle\hat{S}_{uv}\rangle B^a_{\text{eff}}\text{Tr}\left([\hat{S}_{ml},[\hat{S}_{uv},\hat{S}_a]]\hat{S}_n\right)\end{aligned} \tag{13}$$

Here, we have immediately ignored the identity matrix. These terms will not contribute because of $[\hat{\mathbf{1}},\hat{S}_a]=0$.

Let our investigation start with the second and third term. In both cases the double commutator ($[\hat{S}_{ml},[\hat{S}_b,\hat{S}_a]]$ and $[\hat{S}_b,[\hat{S}_{ml},\hat{S}_a]]$) will end up with four terms containing a bivector $\hat{S}_{ab}$. Therefore, the traces $\text{Tr}\left([\hat{S}_{ml},[\hat{S}_b,\hat{S}_a]]\hat{S}_n\right)$ as well as $\text{Tr}\left([\hat{S}_b,[\hat{S}_{ml},\hat{S}_a]]\hat{S}_n\right)$ become zero because $\text{Tr}\left(\hat{S}_{ab}\hat{S}_n\right)=0$ [see Eq. (5)].

The double commutator $[\hat{S}_{ml},[\hat{S}_{uv},\hat{S}_a]]$ in the last (fourth) term of Eq. (13) leads to two commutators of the type

$$[\hat{S}_{ml},\hat{S}_{op}]=\frac{1}{2}\left([\hat{S}_m\hat{S}_l,\hat{S}_o\hat{S}_p]+[\hat{S}_m\hat{S}_l,\hat{S}_p\hat{S}_o]+[\hat{S}_l\hat{S}_m,\hat{S}_o\hat{S}_p]+[\hat{S}_l\hat{S}_m,\hat{S}_p\hat{S}_o]\right)\ . \tag{14}$$

Now, every commutator of these four commutators can be written as e.g.:

$$[\hat{S}_m\hat{S}_l,\hat{S}_o\hat{S}_p]=\hat{S}_m\hat{S}_o[\hat{S}_l,\hat{S}_p]+\hat{S}_m[\hat{S}_l,\hat{S}_o]\hat{S}_p+\hat{S}_o[\hat{S}_m,\hat{S}_p]\hat{S}_l+[\hat{S}_m,\hat{S}_o]\hat{S}_l\hat{S}_p\ . \tag{15}$$

The important point is that we have now two identical sums $\sum_{ml}$ and $\sum_{uv}$. Therefore, we will always find commutator pairs like $[\hat{S}_a,\hat{S}_b]$ and $[\hat{S}_b,\hat{S}_a]=-[\hat{S}_a,\hat{S}_b]$. This means at the end, we have pairs of identical traces: $\text{Tr}\left(\hat{S}_a\hat{S}_b\hat{S}_c\hat{S}_n\right)$ and $-\text{Tr}\left(\hat{S}_a\hat{S}_b\hat{S}_c\hat{S}_n\right)$, just with opposite signs, which neglect each other. Therefore, the sum over all traces gives zero and the last term of Eq. (13) does not contribute to the dynamics of $\langle\hat{S}_n\rangle$.

Let us come to the missing first term of Eq. (13). The traces of this term can be written as:

$$\text{Tr}\left([\hat{S}_m,[\hat{S}_b,\hat{S}_a]]\hat{S}_n\right)=\text{Tr}\left(\hat{S}_m\hat{S}_b\hat{S}_a\hat{S}_n\right)-\text{Tr}\left(\hat{S}_m\hat{S}_a\hat{S}_b\hat{S}_n\right)-\text{Tr}\left(\hat{S}_b\hat{S}_a\hat{S}_m\hat{S}_n\right)+\text{Tr}\left(\hat{S}_a\hat{S}_b\hat{S}_m\hat{S}_n\right)\ . \tag{16}$$

From quantum mechanics we known that $\text{Tr}\left(\hat{S}_a\hat{S}_b\hat{S}_c\hat{S}_d\right)=n_S\left(\delta_{ab}\delta_{cd}+\delta_{ad}\delta_{bc}\right)$, and $n_S=2$ in the case $S=1$. Therefore, $\text{Tr}\left([\hat{S}_m,[\hat{S}_b,\hat{S}_a]]\hat{S}_n\right)$ becomes:

$$\text{Tr}\left([\hat{S}_m,[\hat{S}_b,\hat{S}_a]]\hat{S}_n\right)=4\left(\delta_{an}\delta_{bm}-\delta_{am}\delta_{bn}\right)=4\epsilon_{rab}\epsilon_{rmn}\ . \tag{17}$$

Furthermore:

$$-\frac{\lambda}{4}\sum_{mba}\langle\hat{S}_m\rangle\langle\hat{S}_b\rangle B^a_{\text{eff}}\text{Tr}\left([\hat{S}_m,[\hat{S}_b,\hat{S}_a]]\hat{S}_n\right)=-\lambda\sum_{mba}\langle\hat{S}_m\rangle\langle\hat{S}_b\rangle B^a_{\text{eff}}\epsilon_{abr}\epsilon_{rmn}=-\lambda\left(\langle\hat{\mathbf{S}}\rangle\times\left(\langle\hat{\mathbf{S}}\rangle\times\mathbf{B}_{\text{eff}}\right)\right)_n\ . \tag{18}$$

In summary, again, only the vector term of $\hat{\rho}$ contributes to the equation of motion for $\langle\hat{S}_n\rangle$ and $-\lambda\mathrm{Tr}\left([\hat{\rho},[\hat{\rho},\hat{\mathrm{H}}]]\hat{S}_n\right)$ becomes:

$$-\lambda\mathrm{Tr}\left([\hat{\rho},[\hat{\rho},\hat{\mathrm{H}}]]\hat{S}_n\right) = -\lambda\left(\langle\hat{\mathbf{S}}\rangle\times\left(\langle\hat{\mathbf{S}}\rangle\times\mathbf{B}_{\mathrm{eff}}\right)\right)_n \ . \tag{19}$$

This means in total, Eq. (1) becomes:

$$\frac{\mathrm{d}}{\mathrm{d}t}\langle\hat{S}_n\rangle = \left(\langle\hat{\mathbf{S}}\rangle\times\mathbf{B}_{\mathrm{eff}}\right)_n - \lambda\left(\langle\hat{\mathbf{S}}\rangle\times\left(\langle\hat{\mathbf{S}}\rangle\times\mathbf{B}_{\mathrm{eff}}\right)\right)_n \ , \tag{20}$$

or written as complete vector equation:

$$\frac{\mathrm{d}}{\mathrm{d}t}\langle\hat{\mathbf{S}}\rangle = \langle\hat{\mathbf{S}}\rangle\times\mathbf{B}_{\mathrm{eff}} - \lambda\langle\hat{\mathbf{S}}\rangle\times\left(\langle\hat{\mathbf{S}}\rangle\times\mathbf{B}_{\mathrm{eff}}\right) \ . \tag{21}$$

## II. ALTERNATIVE DERIVATION

In the previous section Eq. (21) has derived by inserting $\hat{\rho}$ [Eq. (2)] in Eq. (1). We have seen that only the vector term of $\hat{\rho}$ contributes to the equation of motion. Therefore, we can immediately make the ansatz:

$$\hat{\rho} \approx \mathbf{P}\cdot\hat{\mathbf{S}} = P_x\hat{S}_x + P_y\hat{S}_y + P_z\hat{S}_z \ , \tag{22}$$

with $\mathbf{P}$ the normalized polarization

$$\mathbf{P} = \frac{\langle\hat{\mathbf{S}}\rangle}{\hbar S} \ . \tag{23}$$

Inserting $\hat{\rho}$ and $\hat{\mathrm{H}} = -\mathbf{B}_{\mathrm{eff}}\cdot\hat{\mathbf{S}}/\hbar$ in the Liouville equation:

$$\frac{\mathrm{d}\hat{\rho}}{\mathrm{d}t} = \frac{i}{\hbar}[\hat{\rho},\hat{\mathrm{H}}] - \frac{\lambda}{\hbar}[\hat{\rho},[\hat{\rho},\hat{\mathrm{H}}]] \ , \tag{24}$$

leads immediately to:

$$\begin{aligned}\frac{\mathrm{d}P_x}{\mathrm{d}t}\hat{S}_x + \frac{\mathrm{d}P_y}{\mathrm{d}t}\hat{S}_y + \frac{\mathrm{d}P_z}{\mathrm{d}t}\hat{S}_z \ &= \ \frac{1}{\hbar}\left(\mathbf{P}\times\mathbf{B}_{\mathrm{eff}}\right)_x\hat{S}_x + \frac{1}{\hbar}\left(\mathbf{P}\times\mathbf{B}_{\mathrm{eff}}\right)_y\hat{S}_y + \frac{1}{\hbar}\left(\mathbf{P}\times\mathbf{B}_{\mathrm{eff}}\right)_z\hat{S}_z \\ &\quad -\lambda\left(\mathbf{P}\times\left(\mathbf{P}\times\mathbf{B}_{\mathrm{eff}}\right)\right)_x\hat{S}_x - \lambda\left(\mathbf{P}\times\left(\mathbf{P}\times\mathbf{B}_{\mathrm{eff}}\right)\right)_y\hat{S}_y - \lambda\left(\mathbf{P}\times\left(\mathbf{P}\times\mathbf{B}_{\mathrm{eff}}\right)\right)_z\hat{S}_z \ .\end{aligned} \tag{25}$$

It is easy to see that this is nothing else as the vector differential equation for the polarization $\mathbf{P}$ spanned with the basis vectors $\hat{S}_z$, $\hat{S}_z$, and $\hat{S}_z$:

$$\frac{\mathrm{d}\mathbf{P}}{\mathrm{d}t} = \frac{1}{\hbar}\mathbf{P}\times\mathbf{B}_{\mathrm{eff}} - \lambda\mathbf{P}\times\left(\mathbf{P}\times\mathbf{B}_{\mathrm{eff}}\right) \ . \tag{26}$$

Here in this section, $\hbar$ has been explicitly taken into account and not set $\hbar = 1$ as before. This gives us the possibility to discuss the dimensions. The polarization $\mathbf{P}$ is dimensionless, because $\hat{\mathbf{S}}$ has the dimension of $\hbar$: $Js$. The $\mathbf{B}_{\mathrm{eff}}$ has the dimension $J$ due to $\hat{\mathrm{H}} = -\mathbf{B}_{\mathrm{eff}}\cdot\hat{\mathbf{S}}/\hbar$. Therefore, both sides of Eq. (26) have the dimension $1/s$ if $\lambda$ has the dimension $1/Js$. This is equal to the Landau-Lifshitz equation. Moreover, $1/\hbar$ has the same dimension as $\gamma/\mu_S$, with $\gamma$ the gyromagnetic ratio and $\mu_S$ the magnetic moment.

## III. SOME REMARKS ABOUT THE COMMUTATOR AND DOUBLE COMMUTATOR

From classical physics we know the general definition of the Poisson bracket:

$$\{F,G\} = \frac{\partial F}{\partial x_\mu}\frac{\partial G}{\partial x_\nu}J_{\mu\nu} \ , \tag{27}$$

with the arbitrary functions $F = F(x_\mu, x_\nu)$ and $G = G(x_\mu, x_\nu)$ and the symplectic matrix $J_{\mu\nu}$. Here, we have already assumed the summation convention, which tells us when an index variable appears twice in a single term it implies summation over all the values of the index of that term.

As a logical consequence of the definition of the Poisson bracket the double Poisson bracket is defined as:

$$\{F,\{G,H\}\} \;=\; \frac{\partial F}{\partial x_\mu}\frac{\partial}{\partial x_\nu}\left(\frac{\partial G}{\partial x_\alpha}\frac{\partial H}{\partial x_\beta}J_{\alpha\beta}\right)J_{\mu\nu}\;. \tag{28}$$

In the case of a spin system $x_\mu$ has to be replaced by $S_n$, and the symplectic matrix $J_{\mu\nu}$ is given by $S_l\epsilon_{nml}$. Therefore, the Poisson bracket becomes:

$$\{\mathcal{F},\mathcal{G}\} = \frac{\partial \mathcal{F}}{\partial S_n}\frac{\partial \mathcal{G}}{\partial S_m}S_l\epsilon_{nml}\;, \tag{29}$$

with $\mathcal{F}=\mathcal{F}(\mathbf{S})$ and $\mathcal{G}=\mathcal{G}(\mathbf{S})$ are arbitrary spin functions.

The corresponding double Poisson bracket is given by:

$$\{\mathcal{F},\{\mathcal{G},\mathcal{H}\}\} = \frac{\partial \mathcal{F}}{\partial S_n}\frac{\partial}{\partial S_m}\left(\frac{\partial \mathcal{G}}{\partial S_a}\frac{\partial \mathcal{H}}{\partial S_b}S_c\right)S_l\epsilon_{abc}\epsilon_{nml}\;. \tag{30}$$

The connection between Poisson bracket $\{\;,\;\}$ and commutator $[\;,\;]$ is given by the transformation $[\;,\;]\leftrightarrow i\hbar\{\;,\;\}$. In the case of the double Poisson bracket: $[\;,[\;,\;]]\leftrightarrow -\hbar^2\{\;,\{\;,\;\}\}$.

Then, we can easily calculate the commutator $[\hat\rho,\hat{\mathrm{H}}]$ and double commutator $[\hat\rho,[\hat\rho,\hat{\mathrm{H}}]$ of the Liouville equation (24) using the definitions for $\hat\rho$ [Eq. (22)] and $\hat{\mathrm{H}}=-B^u_{\mathrm{eff}}\hat S_u/\hbar$:

$$\frac{i}{\hbar}[\hat\rho,\hat{\mathrm{H}}] \;=\; \frac{1}{\hbar}P_uB^v_{\mathrm{eff}}\frac{\partial \hat S_u}{\partial \hat S_n}\frac{\partial \hat S_v}{\partial \hat S_m}\hat S_l\epsilon_{nml} = P_uB^v_{\mathrm{eff}}\hat S_l\delta_{un}\delta_{vm}\epsilon_{nml} = (\mathbf{P}\times\mathbf{B}_{\mathrm{eff}})_l\,\hat S_l\;, \tag{31}$$

$$-\frac{\lambda}{\hbar}[\hat\rho,[\hat\rho,\hat{\mathrm{H}}]] \;=\; -\lambda P_uP_vB^w_{\mathrm{eff}}\frac{\partial \hat S_u}{\partial \hat S_n}\frac{\partial \hat S_v}{\partial \hat S_a}\frac{\partial \hat S_w}{\partial \hat S_b}\frac{\partial \hat S_c}{\partial \hat S_m}\hat S_l\epsilon_{abc}\epsilon_{nml} = -\lambda P_nP_aB^b_{\mathrm{eff}}\hat S_l\epsilon_{abm}\epsilon_{nml} = -\lambda\left(\mathbf{P}\times(\mathbf{P}\times\mathbf{B}_{\mathrm{eff}})\right)_l\hat S_l\;. \tag{32}$$

## IV. REDUCED DENSITY OPERATOR

The reduced density operator was introduced by Dirac in 1930 [3]. While the normal density operator $\hat\rho$ contains the information of the full system $\mathcal{H}=\mathcal{H}_A\otimes\mathcal{H}_B$ the reduced density operator $\hat\rho_A$ only the information about the subsystem $\mathcal{H}_A$. Here, we have assumed that the complete Hilbert space $\mathcal{H}$ can be divided into two subsystems $\mathcal{H}_A$ and $\mathcal{H}_B$, e.g. a single spin $\hat{\mathbf{S}}_n$ and the environment (other spins $j\neq n$ or the lattice). This reduction of information can be an advantage in the description especially for huge systems.

The expectation value of an operator $\hat A$ is given by:

$$\langle\hat A\rangle = \mathrm{Tr}_{ab}\left(\hat\rho(ab)\hat A(a)\right)\;. \tag{33}$$

$\hat\rho(ab)$ is the density operator of the complete system and the trace is explicitly expressed as being evaluated over the two sets of variables $a$ and $b$ belonging to the two sub systems $\mathcal{H}_A$ and $\mathcal{H}_B$. The operator $\hat A(a)$ is independent of $b$ and the trace is just a diagonal sum. Therefore, (33) can be written as:

$$\langle\hat A\rangle = \mathrm{Tr}_a\left(\mathrm{Tr}_b\left[\hat\rho(ab)\right]\hat A(a)\right) = \mathrm{Tr}_a\left(\hat\rho_A(a)\hat A(a)\right)\;, \tag{34}$$

with the reduced density operator:

$$\hat\rho_A(a) = \mathrm{Tr}_b\left[\hat\rho(ab)\right]\;. \tag{35}$$

The reduced density operator $\hat\rho_A$ can be used similar to the normal density operator $\hat\rho$, however $\hat\rho_A$ does not contain the full information of the system. To clarify this point it is favorable to investigate the connection between the full and reduced density operator.

The wave function of our system can be expanded by product states constructed by the orthonormal eigenvectors of the subsystems:

$$|\psi\rangle = \sum_{ij}c_{ij}\left(|a_i\rangle\otimes|b_j\rangle\right)\;. \tag{36}$$

Then, the density operator $\hat{\rho}(ab)$ is given by:

$$\hat{\rho}(ab) = |\psi\rangle\langle\psi| = \sum_{iji'j'} c_{ij}c^{\star}_{i'j'} \left(|a_i\rangle\langle a_{i'}| \otimes |b_j\rangle\langle b_{j'}|\right) \ . \tag{37}$$

The reduced density operator $\hat{\rho}_A(a)$ can be evaluated by the trace over the $b$ variables:

$$\hat{\rho}_A(a) = \mathrm{Tr}_b\left[\hat{\rho}(ab)\right] = \sum_{j''}\sum_{iji'j'} c_{ij}c^{\star}_{i'j'} \left(|a_i\rangle\langle a_i| \otimes \langle b_{j''}|b_j\rangle\langle b_{j'}|b_{j''}\rangle\right) = \sum_{iji'} c_{ij}c^{\star}_{i'j}|a_i\rangle\langle a_{i'}| \ . \tag{38}$$

Here, we have used the orthonormality of the eigenfunctions $|b_j\rangle$: $\langle b_{j''}|b_j\rangle = \delta_{jj''}$ and $\langle b_{j'}|b_{j''}\rangle = \delta_{j'j''}$, further the fact that: $\mathbf{M}\otimes s = s\mathbf{M}$, where $\mathbf{M} = |a_i\rangle\langle a_{i'}|$ is a matrix and $s = \delta_{jj''}\delta_{j'j''} = 1$ resp. 0 a scalar.

For the following discussion it is favorable to make a unitary transformation $\tilde{\rho}_A(a) = U^{+}\hat{\rho}_A(a)U$ to make $\hat{\rho}_A(a)$ diagonal in $|a_i\rangle$ [5]. Such a transformation is always possible and does not change the physics, we just change the underlying coordinate system. With such an unitary transformation, we get:

$$\tilde{\rho}_A(a) = \sum_{ij} |c_{ij}|^2|a_i\rangle\langle a_i| \ . \tag{39}$$

$|c_{ij}|^2$ is the probability to find the system in state $|a_i\rangle$ and at the same time in state $|b_j\rangle$. The summation over all $j$:

$$p_i = \sum_j |c_{ij}|^2 \tag{40}$$

gives the overall probability that the system is in state $|a_i\rangle$ regardless of $|b_j\rangle$. Therefore, $\tilde{\rho}_A(a)$ acts like a normal density operator of a mixed system:

$$\tilde{\rho}_A(a) = \sum_i p_i|a_i\rangle\langle a_i| \ . \tag{41}$$

## V. SOME REMARKS ABOUT PURE AND MIXED DENSITY OPERATORS

In the case of a pure system the density operator is given by:

$$\hat{\rho} = |\psi\rangle\langle\psi| \ , \tag{42}$$

and in the case of a mixed state by:

$$\hat{\rho} = \sum_i p_i|\psi_i\rangle\langle\psi_i| \ . \tag{43}$$

As before, $p_i$ is the probability to find the system in state $|\psi_i\rangle$.

Now, we know, that in the case of a pure system we have:

$$\hat{\rho}^2 = |\psi\rangle\langle\psi|\psi\rangle\langle\psi| = |\psi\rangle\langle\psi| = \hat{\rho} \ , \tag{44}$$

and therefore:

$$\mathrm{Tr}\left(\hat{\rho}^2\right) = \mathrm{Tr}\left(\hat{\rho}\right) = 1 \ . \tag{45}$$

In the case of a mixed state we find:

$$\hat{\rho}^2 = \sum_{ij} p_ip_j|\psi_i\rangle\langle\psi_i|\psi_j\rangle\langle\psi_j| = \sum_i p_i^2|\psi_i\rangle\langle\psi_i| \ . \tag{46}$$

This means:

$$\mathrm{Tr}\left(\hat{\rho}^2\right) = \sum_{ik} p_i^2\langle k|\psi_i\rangle\langle\psi_i|k\rangle = \sum_{ik} p_i^2\langle\psi_i|k\rangle\langle k|\psi_i\rangle = \sum_i p_i^2 \ . \tag{47}$$

We also know that $\sum_i p_i = 1$. However, $p_i^2$ cannot be greater then $p_i$: $0 \le p_i \le 1$. This means that we have $p_i^2 < p_i$, and therefore, in the case of a mixed state:

$$\mathrm{Tr}\left(\hat{\rho}^2\right) < 1 \; . \tag{48}$$

Let us investigate a simple example: one spin with $S = 1/2$. In this case the density operator $\hat{\rho}$ is given by:

$$\hat{\rho} = \frac{1}{2}\left(\hat{\mathbf{1}} + \langle \hat{\boldsymbol{\sigma}} \rangle \cdot \hat{\boldsymbol{\sigma}}\right) \; . \tag{49}$$

$\hat{\boldsymbol{\sigma}} = (\hat{\sigma}_x, \hat{\sigma}_y, \hat{\sigma}_z)$ are the Pauli matrices and $\hat{\mathbf{1}}$ is the identity matrix. Then, we have

$$\begin{aligned}\mathrm{Tr}\left(\hat{\rho}^2\right) &= \frac{1}{4}\mathrm{Tr}\left(\hat{\mathbf{1}} + \langle \hat{\boldsymbol{\sigma}} \rangle \cdot \hat{\boldsymbol{\sigma}}\right)^2 \\ &= \frac{1}{4}\mathrm{Tr}\left(\hat{\mathbf{1}}^2 + \left(\langle \hat{\boldsymbol{\sigma}} \rangle \cdot \hat{\boldsymbol{\sigma}}\right)^2 + \langle \hat{\boldsymbol{\sigma}} \rangle \cdot \hat{\boldsymbol{\sigma}}\right) \; .\end{aligned} \tag{50}$$

We know, $\hat{\mathbf{1}}^2 = \hat{\mathbf{1}}$, $\mathrm{Tr}(\hat{\boldsymbol{\sigma}}) = 0$, and $\mathrm{Tr}(\hat{\sigma}_\alpha^2) = \hat{\mathbf{1}}$ [see Eq. (5)]. Therefore, we get:

$$\mathrm{Tr}\left(\hat{\rho}^2\right) = \mathrm{Tr}\left(\frac{1 + \langle \hat{\sigma}_x \rangle^2 + \langle \hat{\sigma}_y \rangle^2 + \langle \hat{\sigma}_z \rangle^2}{4}\hat{\mathbf{1}}\right) \; . \tag{51}$$

With $\mathrm{Tr}(\hat{\mathbf{1}}) = 2$ in the case of the $2 \times 2$ identity matrix $\hat{\mathbf{1}}$ we get finally:

$$\mathrm{Tr}\left(\hat{\rho}^2\right) = \frac{1 + |\langle \hat{\boldsymbol{\sigma}} \rangle|^2}{2} \le 1 \; , \tag{52}$$

$\mathrm{Tr}\left(\hat{\rho}^2\right) = 1$ in the case of a pure system and $\mathrm{Tr}\left(\hat{\rho}^2\right) < 1$ in the case of a mixed state.

This means we find for a pure state $|\langle \hat{\boldsymbol{\sigma}} \rangle| = 1$ and for a mixed state $|\langle \hat{\boldsymbol{\sigma}} \rangle| < 1$. And, this means that $\langle \hat{\boldsymbol{\sigma}} \rangle$ has a conserved length if the system is in a pure state. In the case of a mixed state $|\langle \hat{\boldsymbol{\sigma}} \rangle|$ depends on the mixture and can vary with the time.

## VI. VON NEUMANN ENTROPY

A good way to quantify the entanglement of a quantum mechanical system is to use the von Neumann entropy:

$$S\left(\hat{\rho}_A\right) = -\mathrm{Tr}\left(\hat{\rho}_A \log_2 \hat{\rho}_A\right) \; . \tag{53}$$

The von Neumann entropy can be seen as the quantum mechanical analog of the classical Shannon entropy known from the information theory [4]. $\hat{\rho}_A$ is the reduced density operator defined before in section IV.

If the system shows no entanglement the von Neumann entropy is zero: $S\left(\hat{\rho}_A\right) = 0$. However, a nonzero value: $S\left(\hat{\rho}_A\right) > 0$ means entanglement. The value of $S\left(\hat{\rho}_A\right)$ increase with increasing entanglement. Alternative to Eq. (53), we can calculate the von Neumann entropy via:

$$S\left(\hat{\rho}_A\right) = -\sum_i \lambda_i \log_2 \lambda_i \; , \tag{54}$$

where $\lambda_i$ are the eigenvalues of $\hat{\rho}_A$: $\det\left(\hat{\rho}_A - \lambda\hat{\mathbf{1}}\right) = 0$.

Please notice: in the case $\lambda_i = 0$ the von Neumann entropy $S\left(\hat{\rho}_A\right)$ becomes:

$$\lim_{\lambda_i \to 0} S\left(\hat{\rho}_A\right) = 0 \; . \tag{55}$$

To get a better understanding the following example shall be discussed: A quantum system with three spins with spin quantum number $S = 1/2$. The wave function in this case is given by:

$$|\psi\rangle = \sum_{m_1 m_2 m_3} c_{m_1 m_2 m_3}\left(|m_1\rangle \otimes |m_2\rangle \otimes |m_3\rangle\right) \; . \tag{56}$$

The basis states $|m_i\rangle = |S_i = \frac{1}{2}, m_i\rangle$, $i \in \{1, 2, 3\}$, can be $|\uparrow\rangle$ or $|\downarrow\rangle$, corresponding to a spin oriented up or down with respect to the quantization axis.

Then the density operator $\hat{\rho}$ of the complete system is given by:

$$\hat{\rho} = |\psi\rangle\langle\psi| = \sum_{m_1 m_2 m_3} \sum_{m_1' m_2' m_3'} c_{m_1 m_2 m_3} c^*_{m_1' m_2' m_3'} \left( |m_1\rangle\langle m_1'| \otimes |m_2\rangle\langle m_2'| \otimes |m_3\rangle\langle m_3'| \right) \ . \tag{57}$$

Or written in matrix form:

$$\hat{\rho} = \begin{pmatrix}
|c_{\uparrow\uparrow\uparrow}|^2 & c_{\uparrow\uparrow\uparrow}c^*_{\uparrow\uparrow\downarrow} & c_{\uparrow\uparrow\uparrow}c^*_{\uparrow\downarrow\uparrow} & c_{\uparrow\uparrow\uparrow}c^*_{\uparrow\downarrow\downarrow} & c_{\uparrow\uparrow\uparrow}c^*_{\downarrow\uparrow\uparrow} & c_{\uparrow\uparrow\uparrow}c^*_{\downarrow\uparrow\downarrow} & c_{\uparrow\uparrow\uparrow}c^*_{\downarrow\downarrow\uparrow} & c_{\uparrow\uparrow\uparrow}c^*_{\downarrow\downarrow\downarrow} \\
c_{\uparrow\uparrow\downarrow}c^*_{\uparrow\uparrow\uparrow} & |c_{\uparrow\uparrow\downarrow}|^2 & c_{\uparrow\uparrow\downarrow}c^*_{\uparrow\downarrow\uparrow} & c_{\uparrow\uparrow\downarrow}c^*_{\uparrow\downarrow\downarrow} & c_{\uparrow\uparrow\downarrow}c^*_{\downarrow\uparrow\uparrow} & c_{\uparrow\uparrow\downarrow}c^*_{\downarrow\uparrow\downarrow} & c_{\uparrow\uparrow\downarrow}c^*_{\downarrow\downarrow\uparrow} & c_{\uparrow\uparrow\downarrow}c^*_{\downarrow\downarrow\downarrow} \\
c_{\uparrow\downarrow\uparrow}c^*_{\uparrow\uparrow\uparrow} & c_{\uparrow\downarrow\uparrow}c^*_{\uparrow\uparrow\downarrow} & |c_{\uparrow\downarrow\uparrow}|^2 & c_{\uparrow\downarrow\uparrow}c^*_{\uparrow\downarrow\downarrow} & c_{\uparrow\downarrow\uparrow}c^*_{\downarrow\uparrow\uparrow} & c_{\uparrow\downarrow\uparrow}c^*_{\downarrow\uparrow\downarrow} & c_{\uparrow\downarrow\uparrow}c^*_{\downarrow\downarrow\uparrow} & c_{\uparrow\downarrow\uparrow}c^*_{\downarrow\downarrow\downarrow} \\
c_{\uparrow\downarrow\downarrow}c^*_{\uparrow\uparrow\uparrow} & c_{\uparrow\downarrow\downarrow}c^*_{\uparrow\uparrow\downarrow} & c_{\uparrow\downarrow\downarrow}c^*_{\uparrow\downarrow\uparrow} & |c_{\uparrow\downarrow\downarrow}|^2 & c_{\uparrow\downarrow\downarrow}c^*_{\downarrow\uparrow\uparrow} & c_{\uparrow\downarrow\downarrow}c^*_{\downarrow\uparrow\downarrow} & c_{\uparrow\downarrow\downarrow}c^*_{\downarrow\downarrow\uparrow} & c_{\uparrow\downarrow\downarrow}c^*_{\downarrow\downarrow\downarrow} \\
c_{\downarrow\uparrow\uparrow}c^*_{\uparrow\uparrow\uparrow} & c_{\downarrow\uparrow\uparrow}c^*_{\uparrow\uparrow\downarrow} & c_{\downarrow\uparrow\uparrow}c^*_{\uparrow\downarrow\uparrow} & c_{\downarrow\uparrow\uparrow}c^*_{\uparrow\downarrow\downarrow} & |c_{\downarrow\uparrow\uparrow}|^2 & c_{\downarrow\uparrow\uparrow}c^*_{\downarrow\uparrow\downarrow} & c_{\downarrow\uparrow\uparrow}c^*_{\downarrow\downarrow\uparrow} & c_{\downarrow\uparrow\uparrow}c^*_{\downarrow\downarrow\downarrow} \\
c_{\downarrow\uparrow\downarrow}c^*_{\uparrow\uparrow\uparrow} & c_{\downarrow\uparrow\downarrow}c^*_{\uparrow\uparrow\downarrow} & c_{\downarrow\uparrow\downarrow}c^*_{\uparrow\downarrow\uparrow} & c_{\downarrow\uparrow\downarrow}c^*_{\uparrow\downarrow\downarrow} & c_{\downarrow\uparrow\downarrow}c^*_{\downarrow\uparrow\uparrow} & |c_{\downarrow\uparrow\downarrow}|^2 & c_{\downarrow\uparrow\downarrow}c^*_{\downarrow\downarrow\uparrow} & c_{\downarrow\uparrow\downarrow}c^*_{\downarrow\downarrow\downarrow} \\
c_{\downarrow\downarrow\uparrow}c^*_{\uparrow\uparrow\uparrow} & c_{\downarrow\downarrow\uparrow}c^*_{\uparrow\uparrow\downarrow} & c_{\downarrow\downarrow\uparrow}c^*_{\uparrow\downarrow\uparrow} & c_{\downarrow\downarrow\uparrow}c^*_{\uparrow\downarrow\downarrow} & c_{\downarrow\downarrow\uparrow}c^*_{\downarrow\uparrow\uparrow} & c_{\downarrow\downarrow\uparrow}c^*_{\downarrow\uparrow\downarrow} & |c_{\downarrow\downarrow\uparrow}|^2 & c_{\downarrow\downarrow\uparrow}c^*_{\downarrow\downarrow\downarrow} \\
c_{\downarrow\downarrow\downarrow}c^*_{\uparrow\uparrow\uparrow} & c_{\downarrow\downarrow\downarrow}c^*_{\uparrow\uparrow\downarrow} & c_{\downarrow\downarrow\downarrow}c^*_{\uparrow\downarrow\uparrow} & c_{\downarrow\downarrow\downarrow}c^*_{\uparrow\downarrow\downarrow} & c_{\downarrow\downarrow\downarrow}c^*_{\downarrow\uparrow\uparrow} & c_{\downarrow\downarrow\downarrow}c^*_{\downarrow\uparrow\downarrow} & c_{\downarrow\downarrow\downarrow}c^*_{\downarrow\downarrow\uparrow} & |c_{\downarrow\downarrow\downarrow}|^2
\end{pmatrix} \ . \tag{58}$$

Only the red matrix elements contribute to the reduced density operator $\hat{\rho}_A = \hat{\rho}_{m_1}$, corresponding to the first spin:

$$\hat{\rho}_{m_1} = \mathrm{Tr}_{m_2 m_3}\left(\hat{\rho}\right) \ . \tag{59}$$

$\mathrm{Tr}_{m_2 m_3}$ is the partial trace over the contributions coming from the second and third spin. All the information, about the system, stored in the black matrix elements get lost during the calculation of the reduced density operator $\hat{\rho}_{m_1}$.

Then, we can write:

$$\begin{aligned}
\hat{\rho}_{m_1} &= \sum_{m_2'' m_3''} \left( \langle m_3''| \otimes \langle m_2''| \right) \hat{\rho} \left( |m_2''\rangle \otimes |m_3''\rangle \right) \\
&= \sum_{m_1 m_2 m_3} \sum_{m_1' m_2' m_3'} \sum_{m_2'' m_3''} c_{m_1 m_2 m_3} c^*_{m_1' m_2' m_3'} \left( |m_1\rangle\langle m_1'| \otimes \langle m_2''|m_2\rangle\langle m_2'|m_2''\rangle \otimes \langle m_3''|m_3\rangle\langle m_3'|m_3''\rangle \right) \\
&= \sum_{m_1 m_1'} \sum_{m_2 m_3} c_{m_1 m_2 m_3} c^*_{m_1' m_2 m_3} |m_1\rangle\langle m_1'| \ .
\end{aligned} \tag{60}$$

All sums are over the possible configurations $\uparrow$ and $\downarrow$. Then we can write the reduced density operator $\hat{\rho}_{m_1}$ in matrix form as:

$$\hat{\rho}_{m_1} = \begin{pmatrix}
|c|^2_{\uparrow\uparrow\uparrow} + |c|^2_{\uparrow\uparrow\downarrow} + |c|^2_{\uparrow\downarrow\uparrow} + |c|^2_{\uparrow\downarrow\downarrow} & c_{\uparrow\uparrow\uparrow}c^*_{\downarrow\uparrow\uparrow} + c_{\uparrow\uparrow\downarrow}c^*_{\downarrow\uparrow\downarrow} + c_{\uparrow\downarrow\uparrow}c^*_{\downarrow\downarrow\uparrow} + c_{\uparrow\downarrow\downarrow}c^*_{\downarrow\downarrow\downarrow} \\
c_{\downarrow\uparrow\uparrow}c^*_{\uparrow\uparrow\uparrow} + c_{\downarrow\uparrow\downarrow}c^*_{\uparrow\uparrow\downarrow} + c_{\downarrow\downarrow\uparrow}c^*_{\uparrow\downarrow\uparrow} + c_{\downarrow\downarrow\downarrow}c^*_{\uparrow\downarrow\downarrow} & |c|^2_{\downarrow\uparrow\uparrow} + |c|^2_{\downarrow\uparrow\downarrow} + |c|^2_{\downarrow\downarrow\uparrow} + |c|^2_{\downarrow\downarrow\downarrow}
\end{pmatrix} \ . \tag{61}$$

Due to the fact that for $S = 1/2$ we have only two configurations up and down the reduced matrix becomes $2 \times 2$. In the case $S = 1$ the matrix would be $3 \times 3$ and so on.

Then, the eigenvalues of this matrix are easily calculated using the standard method: $\det\left(\hat{\rho}_A - \lambda\hat{\mathbf{1}}\right) = 0$. As result we find:

$$\lambda_{1,2} = \frac{\alpha + \delta}{2} \pm \sqrt{\frac{(\alpha+\delta)^2}{4} - (\alpha\delta - \beta\gamma)} \ , \tag{62}$$

with

$$\begin{aligned}
\alpha &= |c|^2_{\uparrow\uparrow\uparrow} + |c|^2_{\uparrow\uparrow\downarrow} + |c|^2_{\uparrow\downarrow\uparrow} + |c|^2_{\uparrow\downarrow\downarrow} \ , \\
\beta &= c_{\uparrow\uparrow\uparrow}c^*_{\downarrow\uparrow\uparrow} + c_{\uparrow\uparrow\downarrow}c^*_{\downarrow\uparrow\downarrow} + c_{\uparrow\downarrow\uparrow}c^*_{\downarrow\downarrow\uparrow} + c_{\uparrow\downarrow\downarrow}c^*_{\downarrow\downarrow\downarrow} \ , \\
\gamma &= c_{\downarrow\uparrow\uparrow}c^*_{\uparrow\uparrow\uparrow} + c_{\downarrow\uparrow\downarrow}c^*_{\uparrow\uparrow\downarrow} + c_{\downarrow\downarrow\uparrow}c^*_{\uparrow\downarrow\uparrow} + c_{\downarrow\downarrow\downarrow}c^*_{\uparrow\downarrow\downarrow} \ , \\
&\text{and} \\
\delta &= |c|^2_{\downarrow\uparrow\uparrow} + |c|^2_{\downarrow\uparrow\downarrow} + |c|^2_{\downarrow\downarrow\uparrow} + |c|^2_{\downarrow\downarrow\downarrow} \ .
\end{aligned}$$

Now, we know $|\psi(t)\rangle$ as function of time $t$. Therefore, we also know $c_{m_1 m_2 m_3}(t)$, $\hat{\rho}(t)$ and $\hat{\rho}_{m_1}(t)$, and with (62), we get the eigenvalues $\lambda_i(t)$ which we need to calculate the von Neumann entropy $S(\hat{\rho}_{m_1}(t))$.

The information loss during reducing the density operator from $\hat{\rho}$ to $\hat{\rho}_{m_1}$ can be seen in the following example: three spins with $S = 1/2$ in the AFM ground state.

In this case the wave function is given by:

$$|\psi\rangle = \frac{1}{\sqrt{2}}\left(|\uparrow\downarrow\uparrow\rangle - |\downarrow\uparrow\downarrow\rangle\right) \, , \tag{63}$$

or in binary code:

$$|\psi\rangle = \frac{1}{\sqrt{2}}\left[\begin{pmatrix}0\\0\\1\\0\\0\\0\\0\\0\end{pmatrix} - \begin{pmatrix}0\\0\\0\\0\\0\\1\\0\\0\end{pmatrix}\right] = \frac{1}{\sqrt{2}}\begin{pmatrix}0\\0\\1\\0\\0\\-1\\0\\0\end{pmatrix} \, . \tag{64}$$

Then, the density operator in matrix form is given by:

$$\hat{\rho} = \frac{1}{2}\begin{pmatrix}0\\0\\1\\0\\0\\-1\\0\\0\end{pmatrix}\begin{pmatrix}0 & 0 & 1 & 0 & 0 & -1 & 0 & 0\end{pmatrix} = \frac{1}{2}\begin{pmatrix}
{\color{red}0} & 0 & 0 & 0 & {\color{red}0} & 0 & 0 & 0\\
0 & {\color{red}0} & 0 & 0 & 0 & {\color{red}0} & 0 & 0\\
0 & 0 & {\color{red}1} & 0 & 0 & -1 & {\color{red}0} & 0\\
0 & 0 & 0 & {\color{red}0} & 0 & 0 & 0 & {\color{red}0}\\
{\color{red}0} & 0 & 0 & 0 & {\color{red}0} & 0 & 0 & 0\\
0 & {\color{red}0} & -1 & 0 & 0 & {\color{red}1} & 0 & 0\\
0 & 0 & {\color{red}0} & 0 & 0 & 0 & {\color{red}0} & 0\\
0 & 0 & 0 & {\color{red}0} & 0 & 0 & 0 & {\color{red}0}
\end{pmatrix} \, . \tag{65}$$

Here, the same color code has been used as before: the red numbers contribute to the reduced density operator $\hat{\rho}_{m_1}$. The information stored in the black matrix elements get lost. The result is:

$$\hat{\rho}_{m_1} = \frac{1}{2}\begin{pmatrix}1 & 0\\0 & 1\end{pmatrix} \, . \tag{66}$$

$\hat{\rho}_{m_1}$ is the reduced density matrix of a single spin (in this case the first spin) in pure spin state with three spins $S = 1/2$. The important point is, $\hat{\rho}_{m_1}$ is identical to the density operator of a mixture with 50% up spins and 50% down spins.

The eigenvalues of this matrix are $\lambda_1 = \lambda_2 = 1/2$, and therefore the von Neumann entropy $S\left(\hat{\rho}_{m_1}\right) = 2(-0.5\log_2 0.5) = 1$, which means that this state is highly entangled.

---


[1] U. Fano, Rev. Mod. Phys **29**, 74 (1957).
[2] V. L. Pokrovsky and N. A. Sinitsyn, Phys. Rev. B **67**, 144303 (2003).
[3] P. A. M. Dirac, Math. Proc. Cambridge Philos. Soc. **26**, 376 (1930).
[4] C. E. Shannon, The Bell System Technical Journal **27**, 379 & 623 (1948).
[5] $U = (\mathbf{v}_1, \ldots, \mathbf{v}_N)$ is a row vector which contains as columns $N$ the eigenvectors $\mathbf{v}_i$ of the density operator $\hat{\rho}_A$ as column vectors.
